# Supplementary material for: AssertionBench: A Benchmark to Evaluate Large-Language Models for Assertion Generation
Source: arXiv:2406.18627 source file (2025-02-28)
Supplement: Supplementary file 1 [file appendix.tex]

\appendix

\section{Appendix}
